# Supplementary material for: Code Prediction by Feeding Trees to Transformers
Source: arXiv:2003.13848 source file (2021-03-08)
Supplement: Supplementary file 1 [file appendix.tex]

\section{Implementation Details}
\label{sec:implementation-details}

\subsection{Modifying the AST}
\label{sec:modifyast}
For the AST, we want the internal AST nodes to only have type information, and the leaf nodes to have value information. This way, our model can predict one information given a node (instead of both type and value). However, in the py150 dataset, there are internal and leaf nodes with both type and value information. To accomodate for this, we slightly modify the trees to fit our definition of ASTs. For nodes with both type and value information, we take the value information, and create a new node (now a leaf node) as the node's first child. Fig~\ref{fig:new_ast} illustrates an example of the modification. This increases the average number of nodes in a tree from 623.4 to 951.9.

\subsection{Splitting Large Trees}
\label{sec:splittrees}
For neural network models, we need to set a maximum number of nodes in the tree that the model can take as input. Ideally, we would want to set the maximum to be high enough to take in any tree of any length; however, in practice, this is infeasible due to memory constraints (and the number of nodes could be infinitely large hypothetically.) We choose the maximum number of context (number of nodes) to be 1000, inspired by the maximum number of context set by GPT2 models and as this covers $> 70\%$ of the training data. For trees with number of nodes greater than 1000, we deploy a technique adopted by \cite{alrfou2018characterlevel}. Given a large tree, we slice it into shorter segments with a sliding window (in our implementation, we used 500, which is half the context). For example, if a tree has 1700 nodes, we would have 3 new shorter trees: from nodes 0-999, nodes 500-1499, and 699-1699. For the last two trees, we would take loss and evaluate only on the nodes that the model has not seen before (1000-1499 and 1500-1699, respectively). In this way, we provide each subsequent shorter segment with some previous context, while increasing the number of training and testing datapoints at a reasonable amount (in our datasets, it doubled the number). An improvement to this sliding window technique would be to maintain the hidden states at each segment to pass along more context information, as explained in \cite{dai2019transformerxl}. 

% \subsection{Why not Positional Encoding?}
% \label{sec:posenc}
% Some Transformers uses positional encoding~\cite{vaswani2017attention} or positional embedding~\cite{radford2019language-gpt2} to provide model extra positional information over elements. However, our early trials with \LeafSeq suggested positional embedding is rather hurting than helping. This is also supported by the claims in \cite{Irie_2019} that positional encoding does not help for language modeling. Thus, we do not use positional encoding or embedding for all our models.
% Recently, \cite{shiv2019novel} tried to introduce tree structures to Transformer models via positional encoding. However, their relative improvement is small compared to what we see with tree-relational prior in Section~\ref{sec:evaluation}.

\begin{figure}
    \centering
    \includegraphics[width=0.5\textwidth]{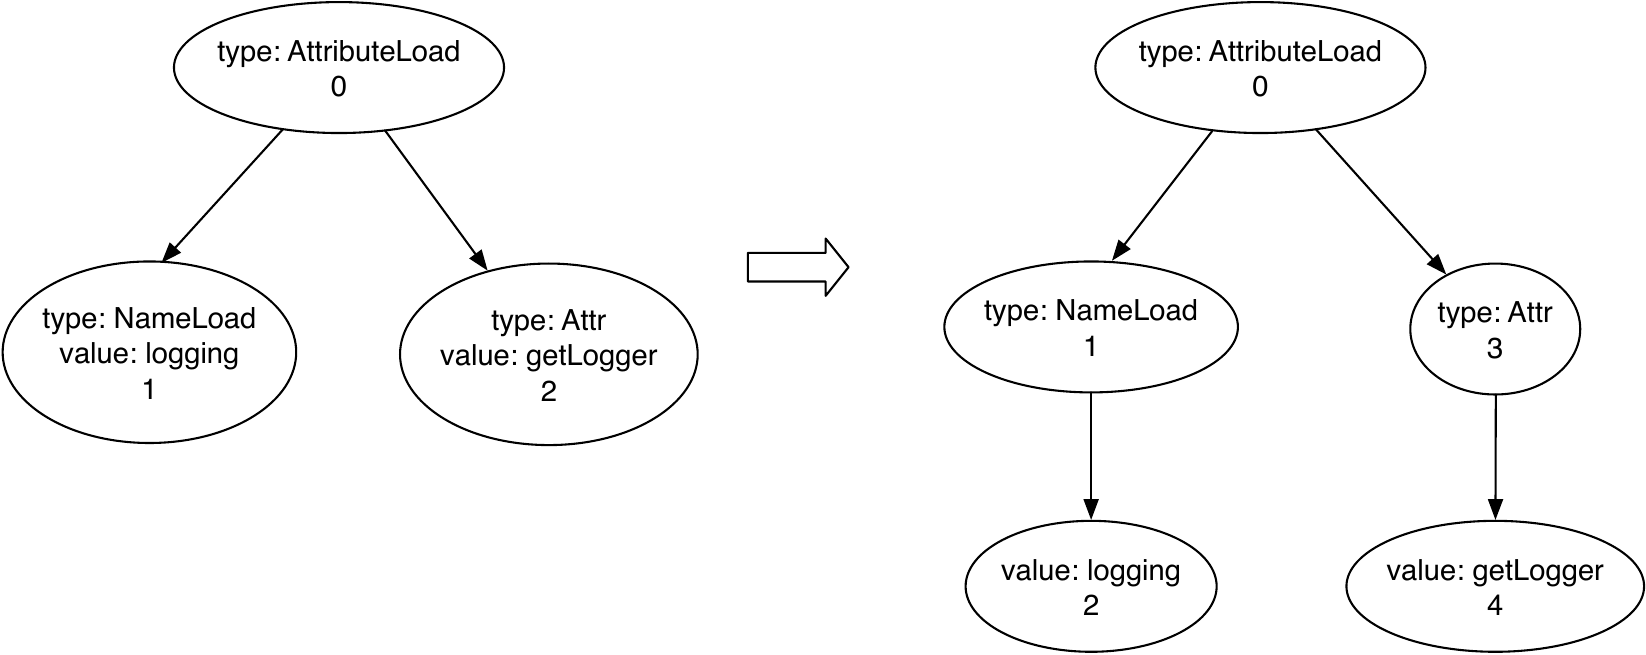}
    \caption{Example AST and our modification to allow nodes to have either only value or type information.}
    \label{fig:new_ast}
\end{figure}
